# Supplementary material for: Ring statistics in 2D-silica: effective temperatures in equilibrium
Source: arXiv:1808.03869 source file (2018-12-07)
Supplement: Supplementary file 1 [file Temperature_deviation_Supporting_info.pdf]

# Supporting Information :

# Ring statistics in 2D-silica: effective temperatures in equilibriuma

Projesh Kumar Roy[1,2] and Andreas Heuer[2]

[1]*NRW Graduate School of Chemistry, Wilhelm-Klemm-Straße 10, 48149 Münster, Germany*

[2]*Institute für Physikalische Chemie, Westfälische-Wilhelms-Universitat Münster, Corrensstraße 28/30, 48149 Münster, Germany*

(Dated: December 6, 2018)

# I. RINGS

## A. Ring Energy

List of all ring energies at $T = 0.015$

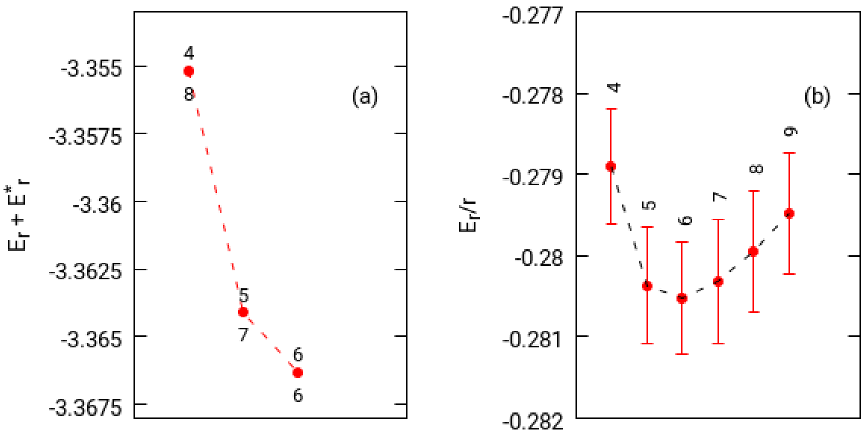


FIG. 1: (a):Complementary ring energies (b):Individual ring energies at $T = 0.015$.

```
#1.Ringsize(r) 2.P_r     3.E_r     4.Standard error
4       0.0514207 -1.11562  0.00286508
5       0.272514  -1.40188  0.0035899
6       0.380929  -1.68315  0.00415416
7       0.225678  -1.96222  0.00539213
8       0.0586961 -2.23954  0.00595436
9       0.0107619 -2.51534  0.00669998
```

## B. Complementary Ring Energy

List of all complementary ring energies at $T = 0.015$.

```
#1.Ringsize(r) 2.Complementary ringsize(r*) 3.P_r*P_r*  4.E_r+E_r*
4       8       0.0030182   -3.35516
5       7       0.0615005   -3.36411
6       6       0.145107    -3.3663
```

## II. TRIPLETS

### A. Triplet Energy

List of all triplet energies at $T = 0.015$.

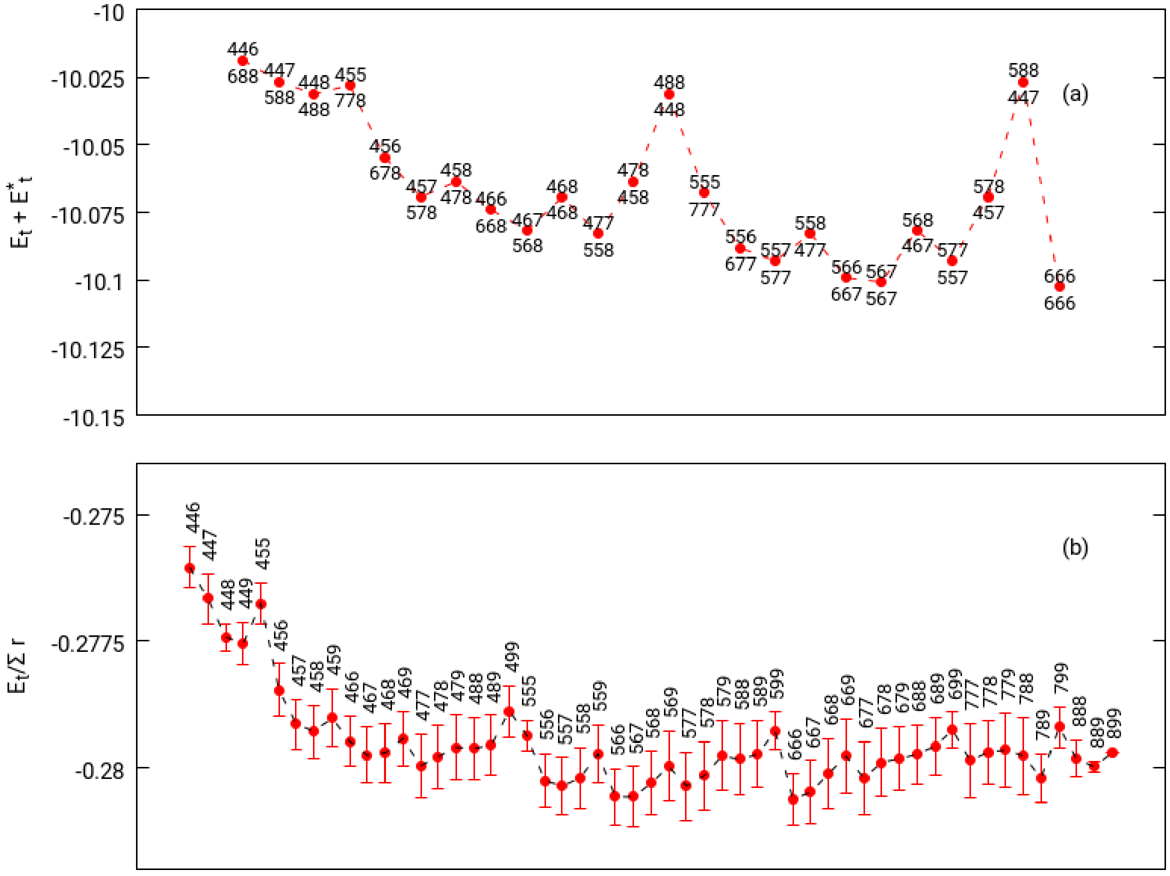


FIG. 2: (a):Complementary triplet energies (b):Individual triplet energies ta $T = 0.015$.

| #1.Triplets | 2.Triplet size(t) | 3.P_t | 4.E_t | 5.Standard_error |
|---|---|---|---|---|
| 444 | 12 | 0 | 0 | 0 |
| 445 | 13 | 0 | 0 | 0 |
| 446 | 14 | 2.34566e-06 | -3.86466 | 0.00551476 |
| 447 | 15 | 6.09871e-05 | -4.15006 | 0.00756095 |
| 448 | 16 | 7.89704e-05 | -4.43875 | 0.00425072 |
| 449 | 17 | 3.90943e-05 | -4.71837 | 0.00707409 |
| 455 | 14 | 2.85388e-05 | -3.87483 | 0.0056482 |

| | | | | |
|---|---|---|---|---|
| 456 | 15 | 0.00101919 | -4.17697 | 0.00766155 |
| 457 | 16 | 0.0035482 | -4.46627 | 0.00798055 |
| 458 | 17 | 0.00403336 | -4.74788 | 0.00895043 |
| 459 | 18 | 0.00225574 | -5.02242 | 0.0102679 |
| 466 | 16 | 0.00552871 | -4.47171 | 0.00798104 |
| 467 | 17 | 0.0228799 | -4.75579 | 0.00938428 |
| 468 | 18 | 0.0144774 | -5.03472 | 0.0104064 |
| 469 | 19 | 0.00507209 | -5.30915 | 0.0103001 |
| 477 | 18 | 0.0166217 | -5.03933 | 0.0113617 |
| 478 | 19 | 0.0159282 | -5.31587 | 0.0119272 |
| 479 | 20 | 0.005542 | -5.59197 | 0.012928 |
| 488 | 20 | 0.00352591 | -5.59243 | 0.0123325 |
| 489 | 21 | 0.001882 | -5.87074 | 0.012359 |
| 499 | 22 | 0.000135657 | -6.13549 | 0.0110973 |
| 555 | 15 | 0.000638409 | -4.19063 | 0.00435124 |
| 556 | 16 | 0.022202 | -4.48411 | 0.00845144 |
| 557 | 17 | 0.0382748 | -4.76614 | 0.00947329 |
| 558 | 18 | 0.0218994 | -5.04364 | 0.010711 |
| 559 | 19 | 0.00458732 | -5.31485 | 0.0107902 |
| 566 | 17 | 0.0879257 | -4.76984 | 0.00928736 |
| 567 | 18 | 0.202056 | -5.0504 | 0.0107195 |
| 568 | 19 | 0.0657042 | -5.32589 | 0.0118657 |
| 569 | 20 | 0.0110891 | -5.59958 | 0.0137708 |
| 577 | 19 | 0.0743022 | -5.32684 | 0.0127174 |
| 578 | 20 | 0.0393542 | -5.60309 | 0.0134692 |
| 579 | 21 | 0.00730085 | -5.87513 | 0.0143146 |
| 588 | 21 | 0.00499351 | -5.87651 | 0.0148443 |
| 589 | 22 | 0.0017006 | -6.15412 | 0.0145215 |
| 599 | 23 | 0.000103991 | -6.42341 | 0.00853014 |
| 666 | 18 | 0.0715319 | -5.05123 | 0.00906692 |
| 667 | 19 | 0.132147 | -5.32933 | 0.0118797 |
| 668 | 20 | 0.0264434 | -5.60236 | 0.0135021 |

| | | | | |
|---|---|---|---|---|
| 669 | 21 | 0.00336523 | -5.87528 | 0.0151893 |
| 677 | 20 | 0.0485355 | -5.60407 | 0.0143169 |
| 678 | 21 | 0.0187809 | -5.8778 | 0.0143198 |
| 679 | 22 | 0.00355641 | -6.15609 | 0.0139853 |
| 688 | 22 | 0.00137846 | -6.15419 | 0.0127658 |
| 689 | 23 | 0.000599706 | -6.43033 | 0.0130258 |
| 699 | 24 | 1.79834e-05 | -6.70225 | 0.00842468 |
| 777 | 21 | 0.00482736 | -5.87716 | 0.0155143 |
| 778 | 22 | 0.00241368 | -6.15321 | 0.0138039 |
| 779 | 23 | 0.000691968 | -6.43196 | 0.0166288 |
| 788 | 23 | 0.000615344 | -6.43462 | 0.0175718 |
| 789 | 24 | 0.000209545 | -6.725 | 0.0117655 |
| 799 | 25 | 6.25508e-06 | -6.98008 | 0.00990649 |
| 888 | 24 | 7.93614e-05 | -6.71594 | 0.00855007 |
| 889 | 25 | 6.64602e-06 | -6.99958 | 0.00237439 |
| 899 | 26 | 1.17283e-06 | -7.27231 | 1.76383e-06 |
| 999 | 27 | 0 | 0 | 0 |

### B. Complementary Triplet Energy

List of all complementary triplet energies at $T = 0.015$.

| #1.Triplet size(t) | 2.Complementary triplet size(t*) | 3.P_tP_t* | 4.E_t+E_t* |
|---|---|---|---|
| 446 | 688 | 3.2334e-09 | -10.0188 |
| 447 | 588 | 3.04539e-07 | -10.0266 |
| 448 | 488 | 2.78443e-07 | -10.0312 |
| 455 | 778 | 6.88836e-08 | -10.028 |
| 456 | 678 | 1.91412e-05 | -10.0548 |
| 457 | 578 | 0.000139637 | -10.0694 |
| 458 | 478 | 6.4244e-05 | -10.0637 |
| 466 | 668 | 0.000146198 | -10.0741 |
| 467 | 568 | 0.00150331 | -10.0817 |
| 468 | 468 | 0.000209595 | -10.0694 |
| 477 | 558 | 0.000364006 | -10.083 |
| 478 | 458 | 6.4244e-05 | -10.0637 |
| 488 | 448 | 2.78443e-07 | -10.0312 |
| 555 | 777 | 3.08183e-06 | -10.0678 |
| 556 | 677 | 0.00107759 | -10.0882 |
| 557 | 577 | 0.0028439 | -10.093 |
| 558 | 477 | 0.000364006 | -10.083 |
| 566 | 667 | 0.0116191 | -10.0992 |
| 567 | 567 | 0.0408265 | -10.1008 |
| 568 | 467 | 0.00150331 | -10.0817 |
| 577 | 557 | 0.0028439 | -10.093 |
| 578 | 457 | 0.000139637 | -10.0694 |
| 588 | 447 | 3.04539e-07 | -10.0266 |
| 666 | 666 | 0.00511682 | -10.1025 |

## III. EFFECTIVE TEMPERATURE FROM TOTAL PROBABILITIES

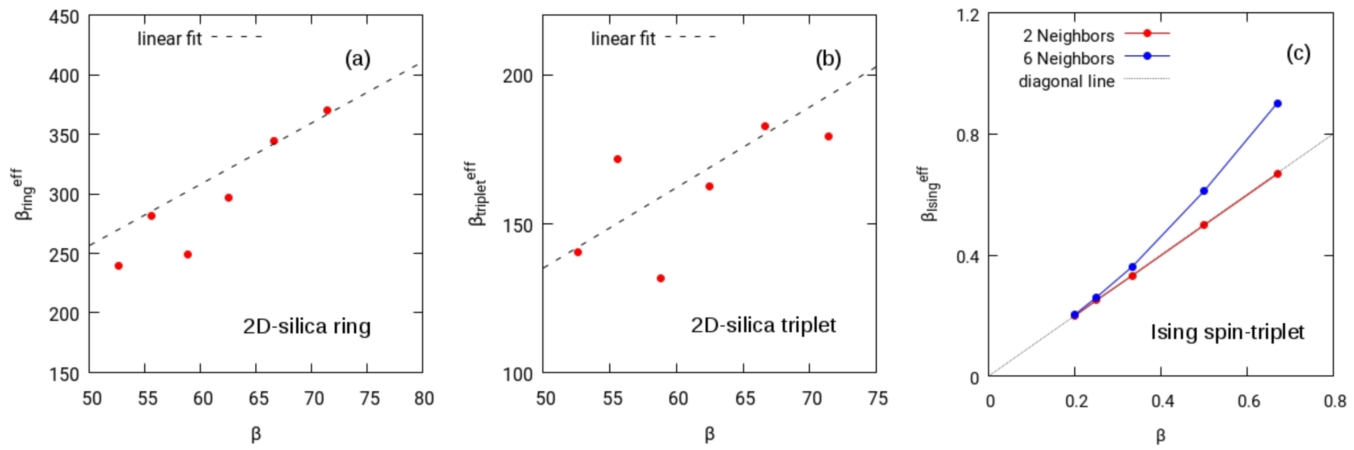


FIG. 3: Variation of (a):$\beta^{eff}_{ring}$ (b):$\beta^{eff}_{triplet}$ and (c):$\beta^{eff}_{Ising}$ with inverse temperature ($\beta$). Data in (a) and (b) are fitted with y = cx where c = 5.1 and 2.7, respectively.

## IV. TEMPERATURE DISTRIBUTION

Following the notation in Ref. [1] we have used the temperature distribution

$$p_{eq}(\beta) = \frac{\exp(-\beta\zeta)\beta^{\lambda_{Dixit}}\zeta^{\lambda_{Dixit}+1}}{\Gamma(\lambda_{Dixit}+1)} \tag{1}$$

to describe the data in Fig.4(a). One can easily show that the standard deviation of the inverse temperature distribution relative to the average inverse temperature is given by $1/\sqrt{1+\lambda_{Dixit}}$. Thus, the value of $\lambda_{Dixit}$ contains the key information to express the relevance of a distribution of temperatures as compared to a single temperature. Note that a graph in Fig.4(a) contains three data points which is identical to the number of free parameters in the problem ($\zeta$, $\lambda_{Dixit}$, and an overall proportionality factor). Thus, the estimation of $\lambda_{Dixit}$ has to be regarded with great caution.

One might speculate that the apparent relevance of some temperature distribution in the low-temperature limit might be related to the deviations from Gaussian behavior due to the increasing relevance of the cutoff of the potential energy landscape in the population of states [3].

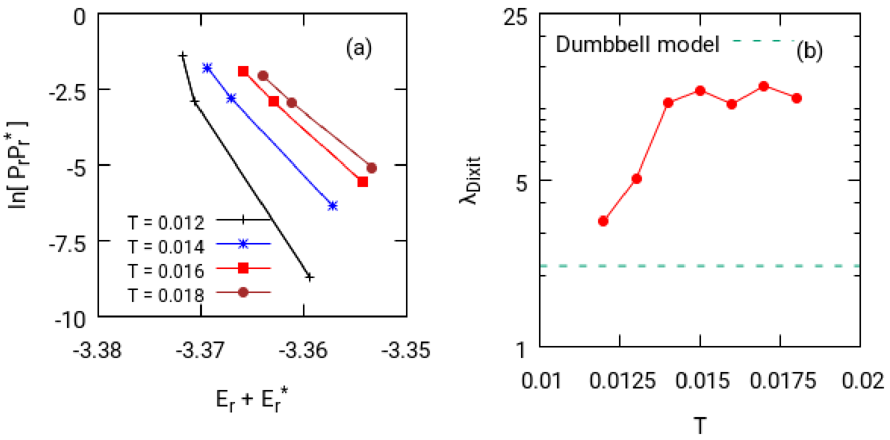


FIG. 4: (a): Plot for logarithm of complementary probabilities vs energies at different temperatures. (b) Estimated $\lambda_{Dixit}$ values from the temperature distribution, provided in reference 1, 2. The line corresponds to the numerical result for the dumbbell in [1].

## V. ISING MODEL

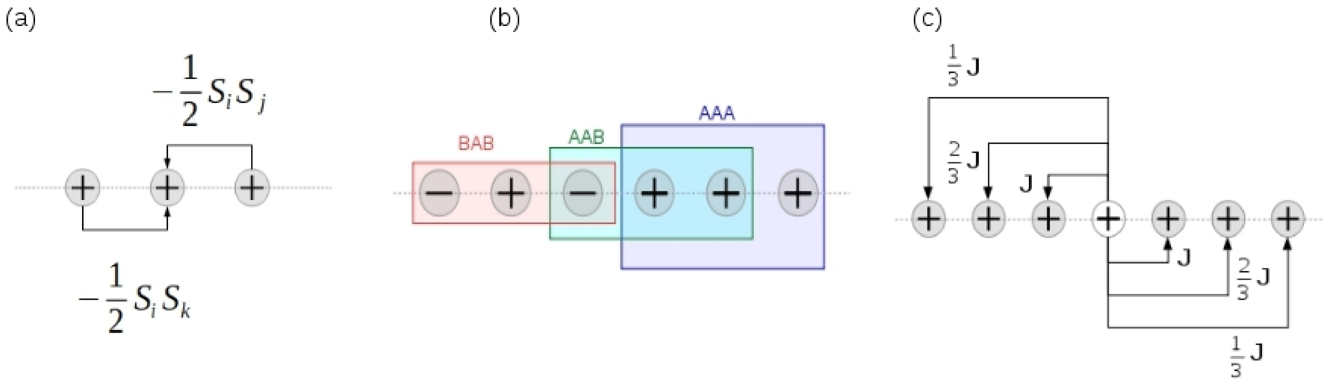


FIG. 5: (a) Defining the energy of a spin from the contributions of its neighbors. (b) Dividing the 1D spin-grids into multiple triplets of spins. (c) Sketch of 1D-Ising model with 3 interacting neighbors on each side.

The degeneracy factors emerge from the equivalence of AAA with BBB, BAB with ABA, and AAB with BBA, BAA, and ABB.

## VI. TOTAL DENSITY OF STATES

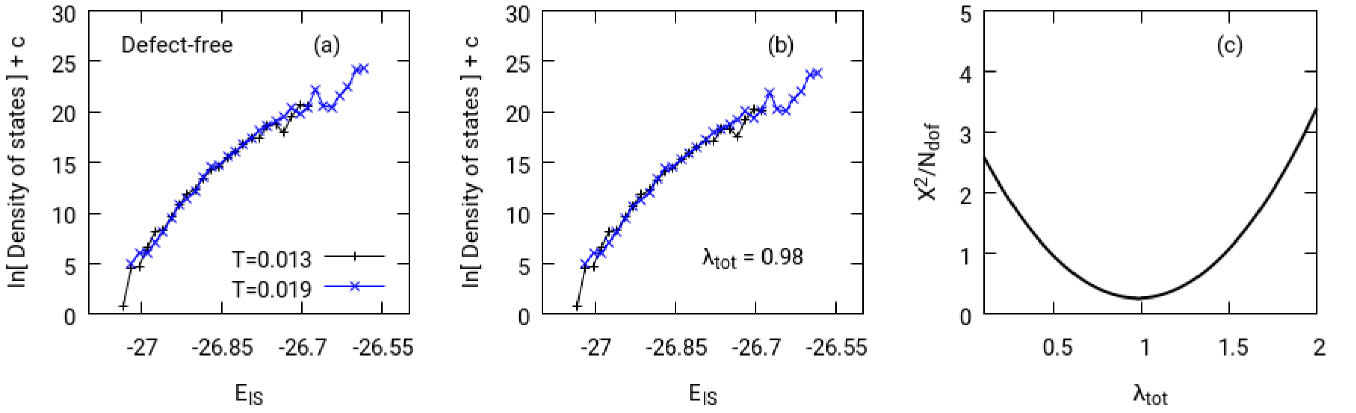


FIG. 6: Logarithm of the density of states plots for defect-free states for $T = 0.013$ and $T = 0.019$ of the *total* system. $E_{IS}$ denotes the energy of the inherent structure. For (a), reweighting is performed with $\beta^{eff} = \beta$. For (b), reweighting is performed with $\beta^{eff} = \lambda_{tot}\beta$ with $\lambda_{tot} = 0.98$. In (c), the variation of reduced $\chi^2(\lambda_{tot})$ (obtained from reweighting in (b) with gnuplot [4]) with $(\lambda_{tot})$ is shown. The minimum $\chi^2$ value corresponds to $\lambda_{tot} = 0.98 \sim 1$.

## VII. DENSITY OF STATES FOR INDIVIDUAL RINGS

The density of states distribution for all ring sizes is determined via reweighting for all probabilities larger than 0.002. For higher energies, anharmonic effects set in which no longer allow a reconstruction via Boltzmann reweighting [5].

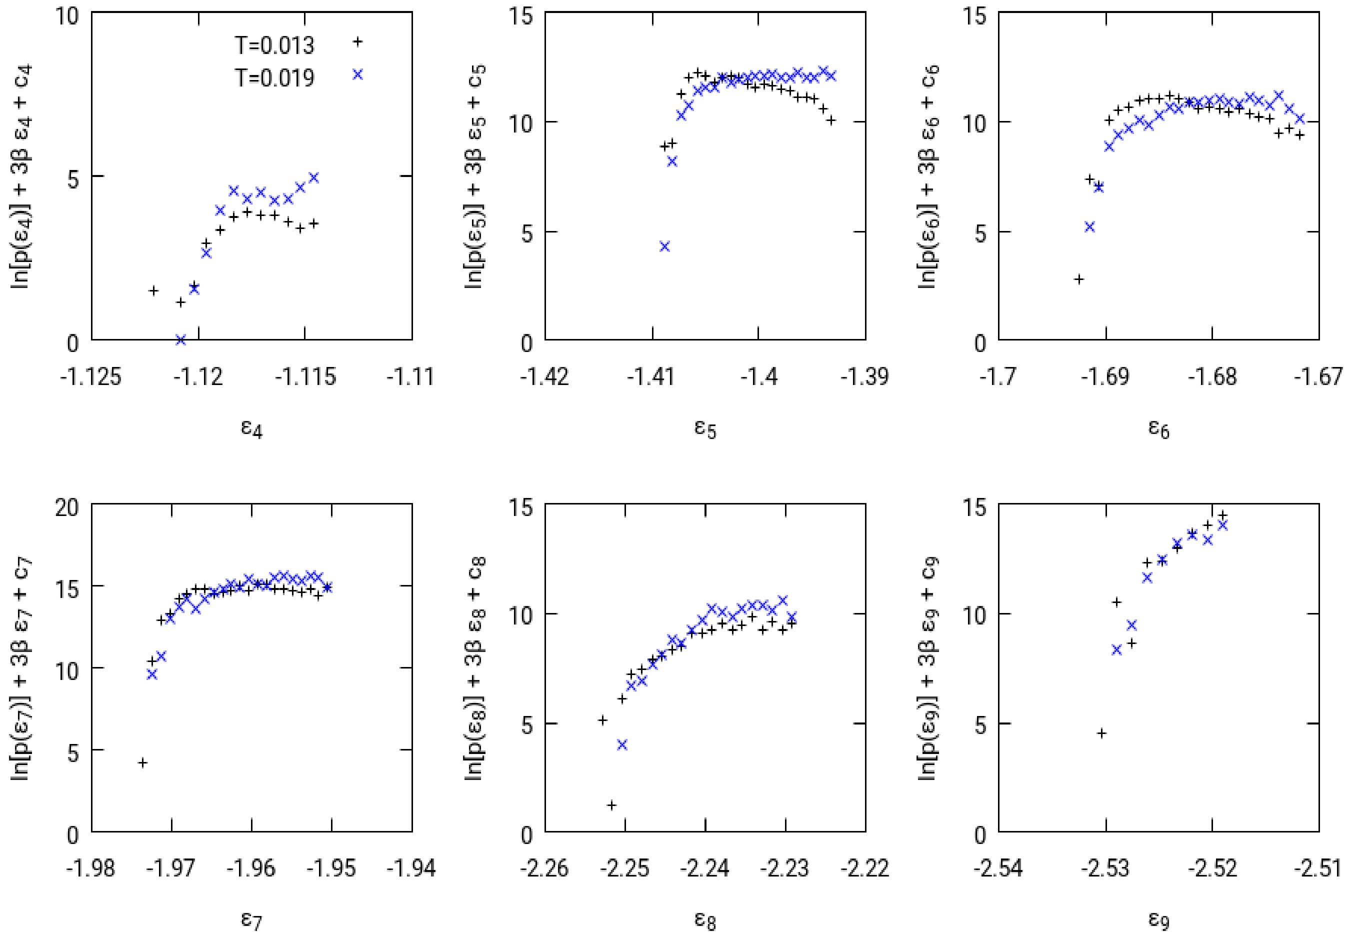


FIG. 7: Logarithm of density of states for (a)4-,(b)5-,(c)6-,(d)7-,(e)8-,(f)9-rings obtained from Boltzmann reweighting with the actual temperature, scaled with a trivial factor of 3. The '$c$' values represent the shift parameters, which are obtained through fitting.

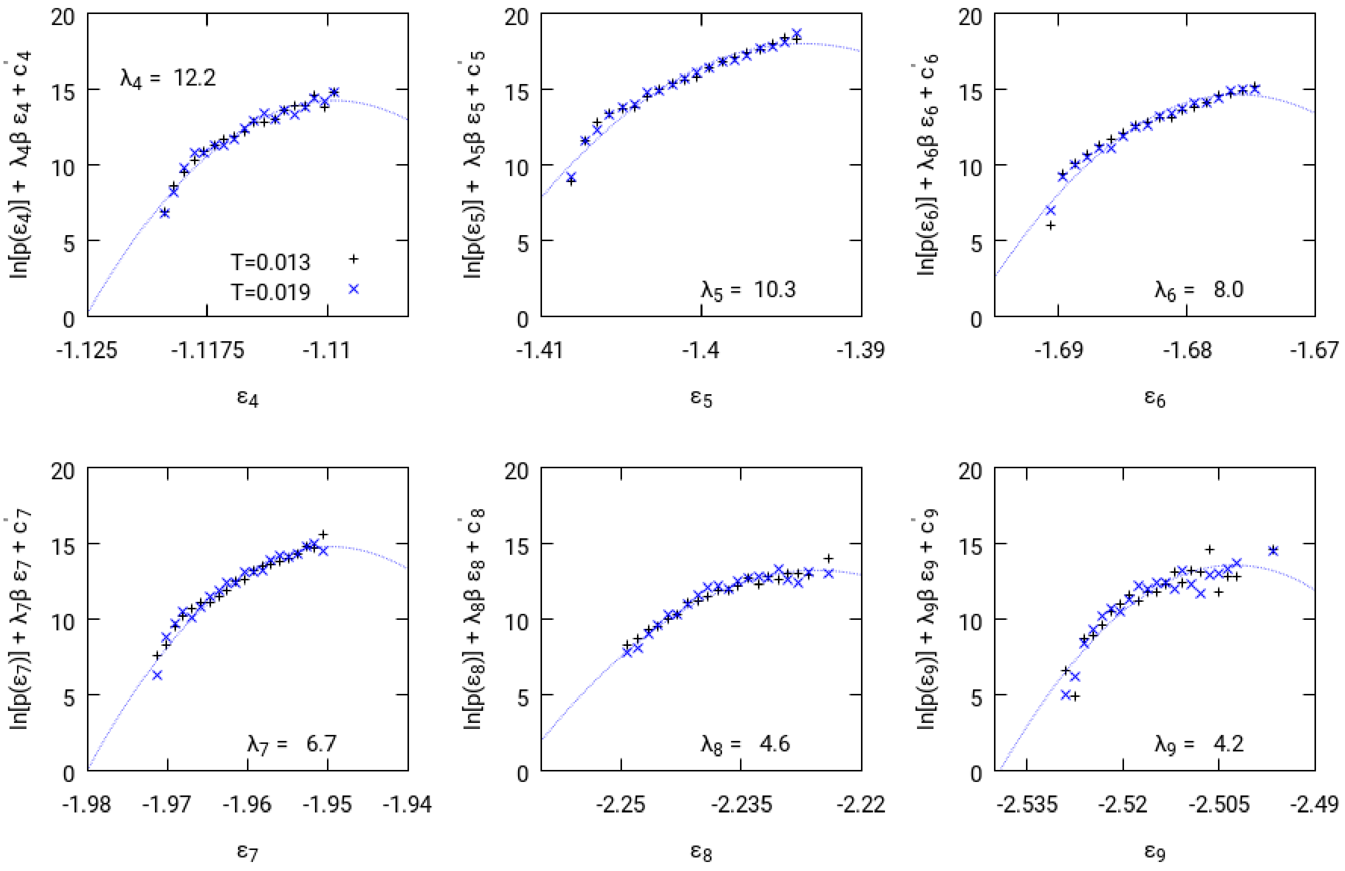


FIG. 8: Logarithm of density of states for (a)4-,(b)5-,(c)6-,(d)7-,(e)8-,(f)9-rings obtained from Boltzmann reweighting with an effective inverse temperature $\lambda^r\beta$. Plots are obtained for a minimum value of reduced $\chi^2(\lambda^r)$, obtained from reweighting between $T = 0.013$ and $T = 0.019$ (see main paper, Fig. 3c). The '$c'$' values represent the shift parameters. All data are plotted where probabilities for both temperatures are greater than 0.002. For ring size 9, probability limit is 0.001.

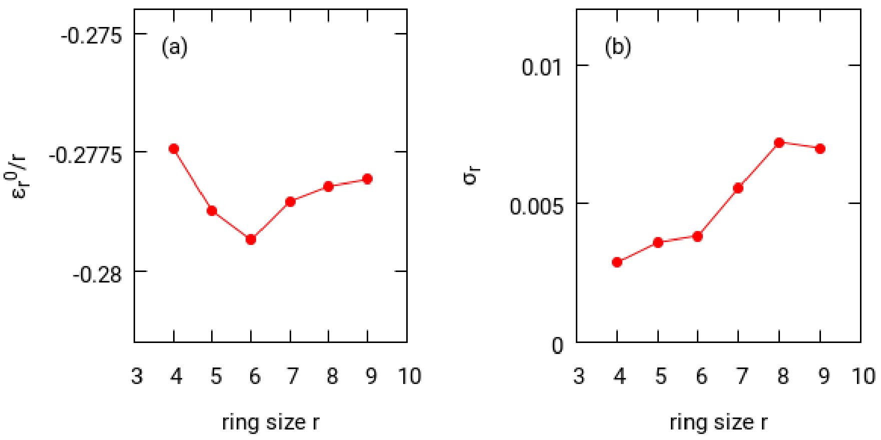


FIG. 9: From a Gaussian fit for the data in Fig. 8 with $g_r(\epsilon_r) \propto \exp\left[-(\epsilon_r - \epsilon_r^0)^2/2\sigma_r^2\right]$, we get (a) $\epsilon_r^0/r$ and (b) $\sigma_r$ for different rings.

## VIII. EXTENDED MODEL ANALYSIS

Generalizing the model from the main part, we consider N subsystems. We assume that all energies $e_i$ and $e_j$ $(i, j \in \{1, ..., N\}, i \neq j)$ are correlated with the same correlation coefficient $\nu$, i.e. $\nu = \langle e_i e_j \rangle / \sigma^2$. This can be realized when assuming that the energies $e_i$ can be written as

$$e_i = B + \epsilon_i \tag{2}$$

where $B$ and $\epsilon_i$ are Gaussian random numbers with variance $b^2$ and $\epsilon^2$, respectively. All $\epsilon_i$ are uncorrelated among each other. The variance $\sigma^2$ of the each subsystem is given by $b^2 + \epsilon^2$.

Of course, in reality the degree of correlation would depend on the distance between two subsystems. Qualitatively, the value of N can be identified with the effective size for which correlations are relevant and $\nu$ is related to the average correlation of pairs of subunits within this volume. The probability to observe a given value of $B$ together with energies $\{e_i\}$ is given by

$$G(B, e_1, ..., e_N) \propto \exp\left[-\frac{B^2}{2b^2}\right] \exp\left[-\frac{(e_1 - B)^2}{2\epsilon^2}\right] ... \exp\left[-\frac{(e_N - B)^2}{2\epsilon^2}\right]. \tag{3}$$

Then the probability to observe energies $e_1, ..., e_N$ in thermal equilibrium can be written as

$$p(e_1, ..., e_N) \propto \int dB\, G(B, e_1, ..., e_N) \exp\left[-\beta(e_1 + ... + e_N)\right]. \tag{4}$$

Of interest is the dependence of the probability $p(e_1, ..., e_M)$ of the energies of a unit of $M$ randomly chosen subsystems (which, without loss of generality, can be chosen as subsystems $1, ...M$). It can be written as

$$p(e_1, ..., e_M) \propto \int de_{M+1} \ldots de_N\, p(e_1, ..., e_N). \tag{5}$$

The underlying Gaussian integrals can be solved in a straightforward manner by quadratic expansion. Before performing the final intergral over $B$, the relevant terms of the total expression read

$$p(e_1, ..., e_M) \propto \int dB \, \exp\left[-\frac{B^2(Mb^2+\epsilon^2)}{2b^2\epsilon^2}\right] \exp\left[B\left(\frac{e_{tot}}{\epsilon^2} - (N-M)\beta\right)\right] \exp\left[-\beta e_{tot}\right]. \quad (6)$$

with $e_{tot} = e_1 + ... + e_M$.

Final integration yields

$$p(e_1, ..., e_M) \propto \exp\left[-\beta e_{tot}\left(1 + \frac{N-M}{M-1+1/\nu}\right)\right]. \quad (7)$$

Thus, the distribution just depends on the sum of the $M$ energy values $e_1, ..., e_M$. This relation is used in the main text.


[1] P. D. Dixit, Phys. Chem. Chem. Phys. **17**, 13000 (2015).

[2] P. D. Dixit, The Journal of Chemical Physics **138**, 184111 (2013).

[3] P. K. Roy, M. Heyde, and A. Heuer, Phys. Chem. Chem. Phys. **20**, 14725 (2018).

[4] T. Williams, C. Kelley, and many others, "Gnuplot 4.6: an interactive plotting program," `http://gnuplot.sourceforge.net/` (2013).

[5] S. Büchner and A. Heuer, Phys. Rev. E. **60**, 6507 (1999).
